# Supplementary material for: What's color got to do with it? Face recognition in grayscale
Source: arXiv:2309.05180 source file (2024-07-03)
Supplement: Supplementary file 1 [file weight__vis_suppl.tex]

\begin{figure*}[ht!]
 \centering
  \begin{subfigure}[b]{\linewidth}
      \begin{subfigure}[b]{0.325\linewidth}
        \centering
          \includegraphics[width=1\linewidth]{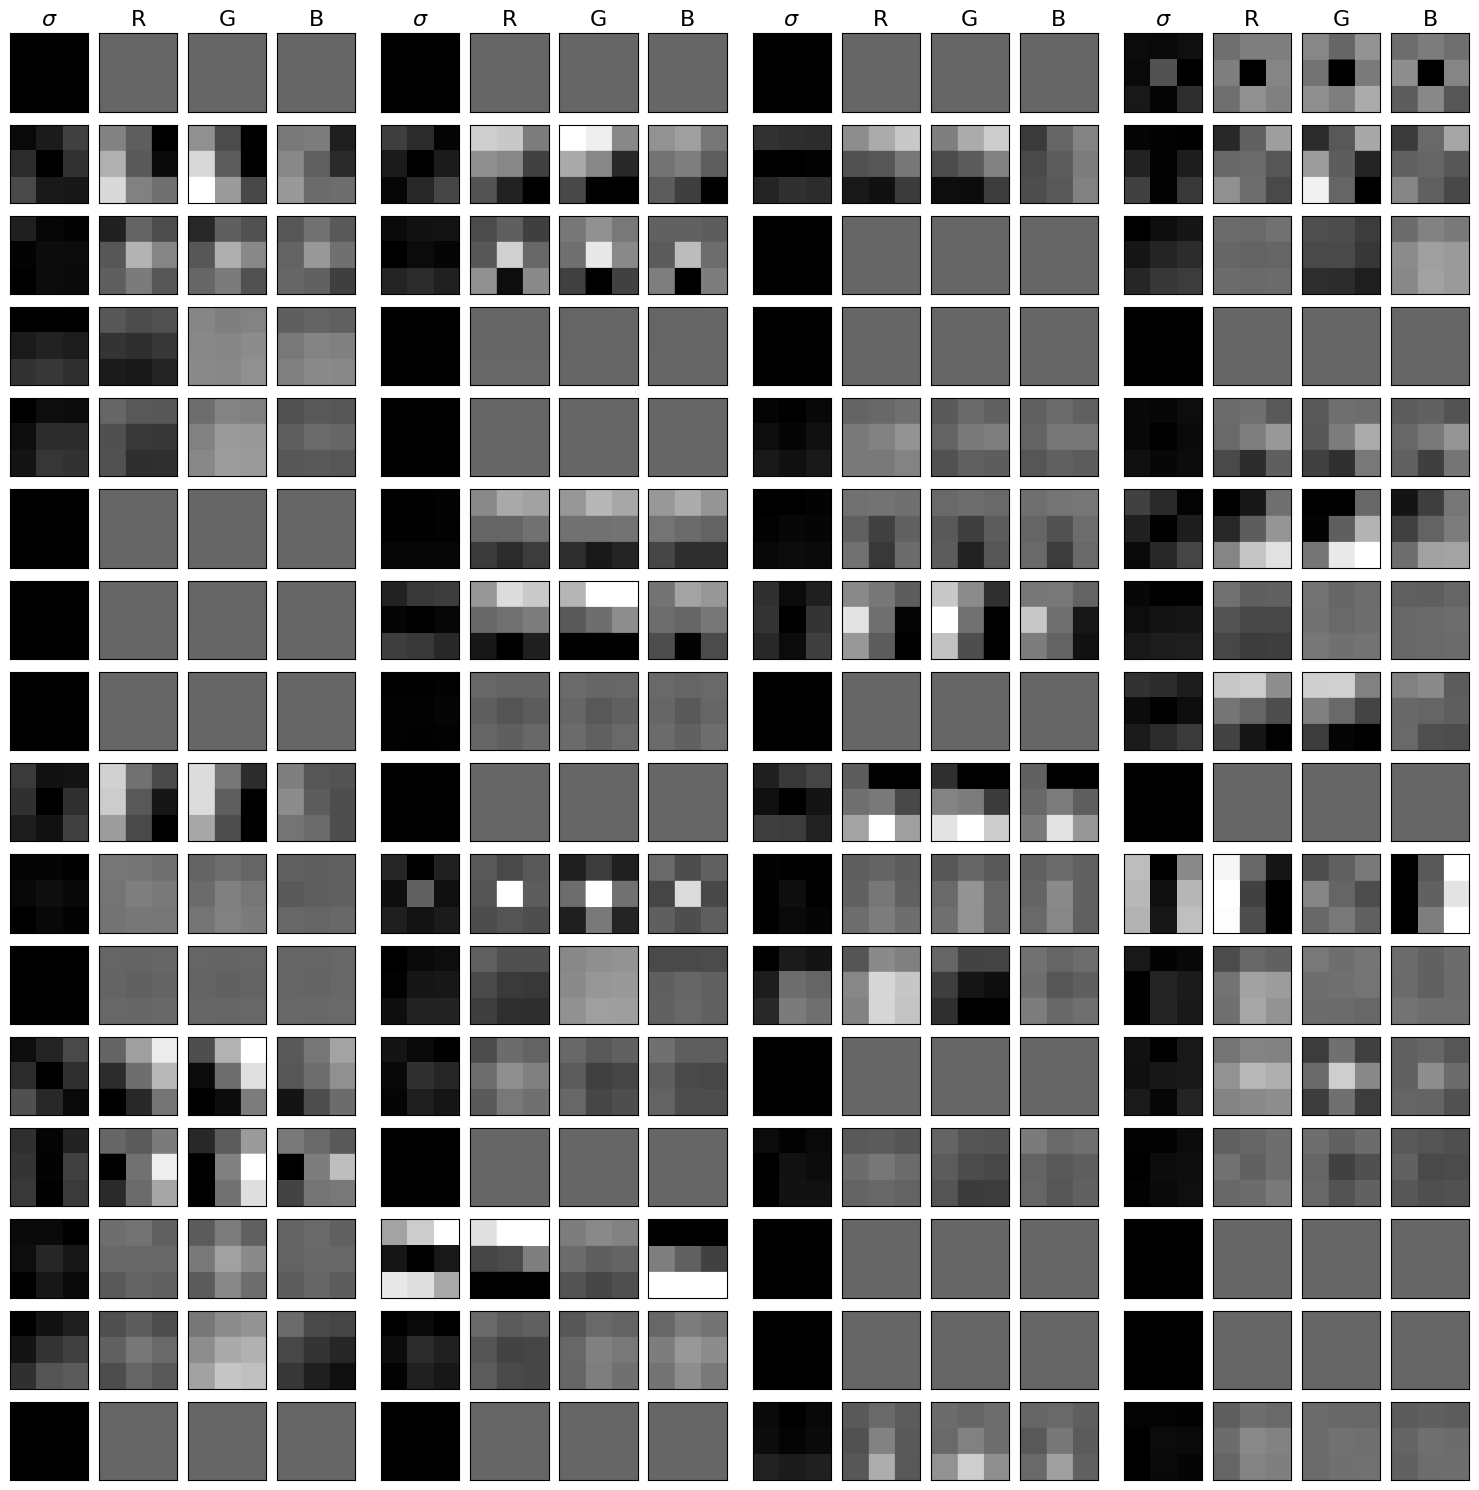}
          \caption{\scriptsize{R18 ``color-cleaned" WebFace4M (RGB)}}\label{wf4mrgb}
        \vspace{0.5em}
      \end{subfigure}
      \hfill
      \begin{subfigure}[b]{0.325\linewidth}
        \centering
          \includegraphics[width=1\linewidth]{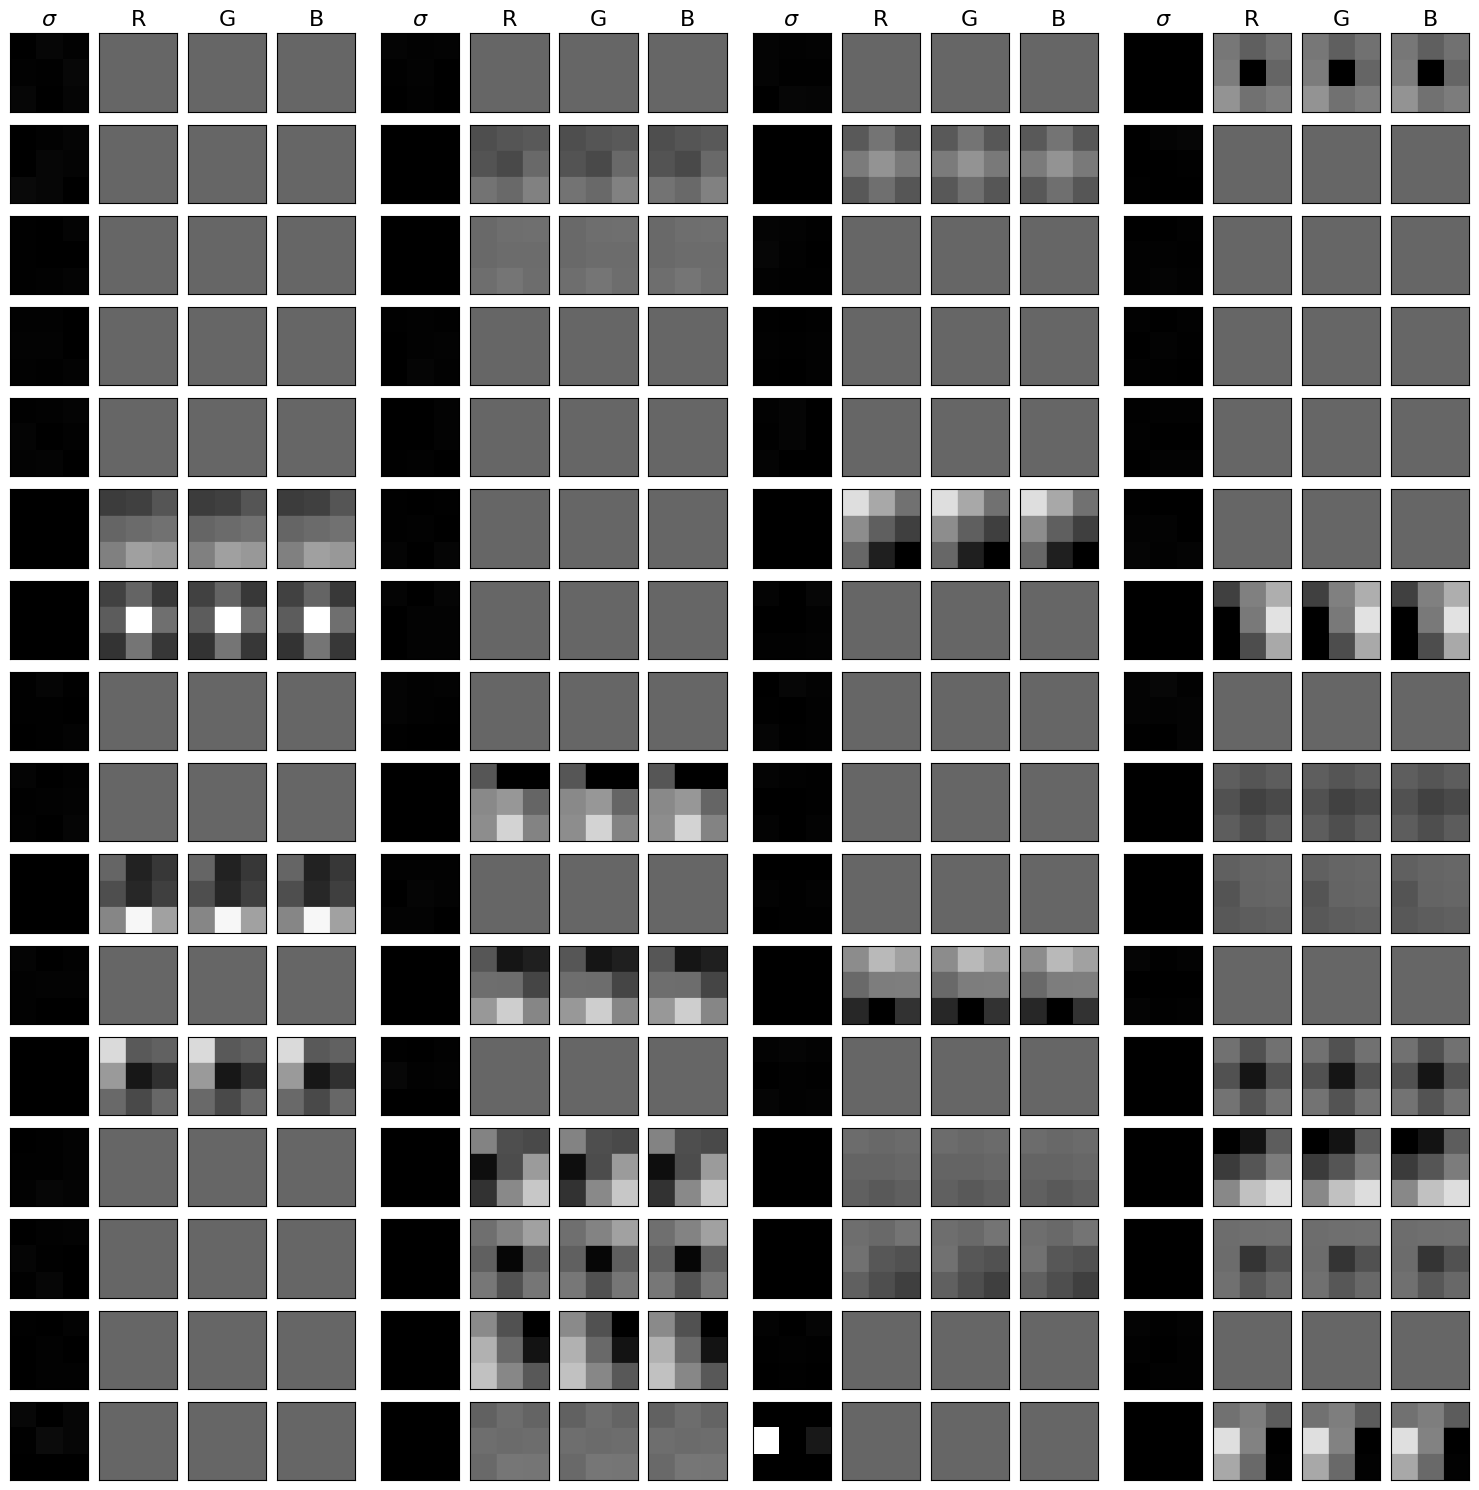}
          \caption{\scriptsize{R18 ``color-cleaned" WebFace4M (Gray 3-channel)}}\label{wf4mgray}
          \vspace{0.5em}
      \end{subfigure}
      \hfill
      \begin{subfigure}[b]{0.325\linewidth}
        \centering
          \includegraphics[width=1\linewidth]{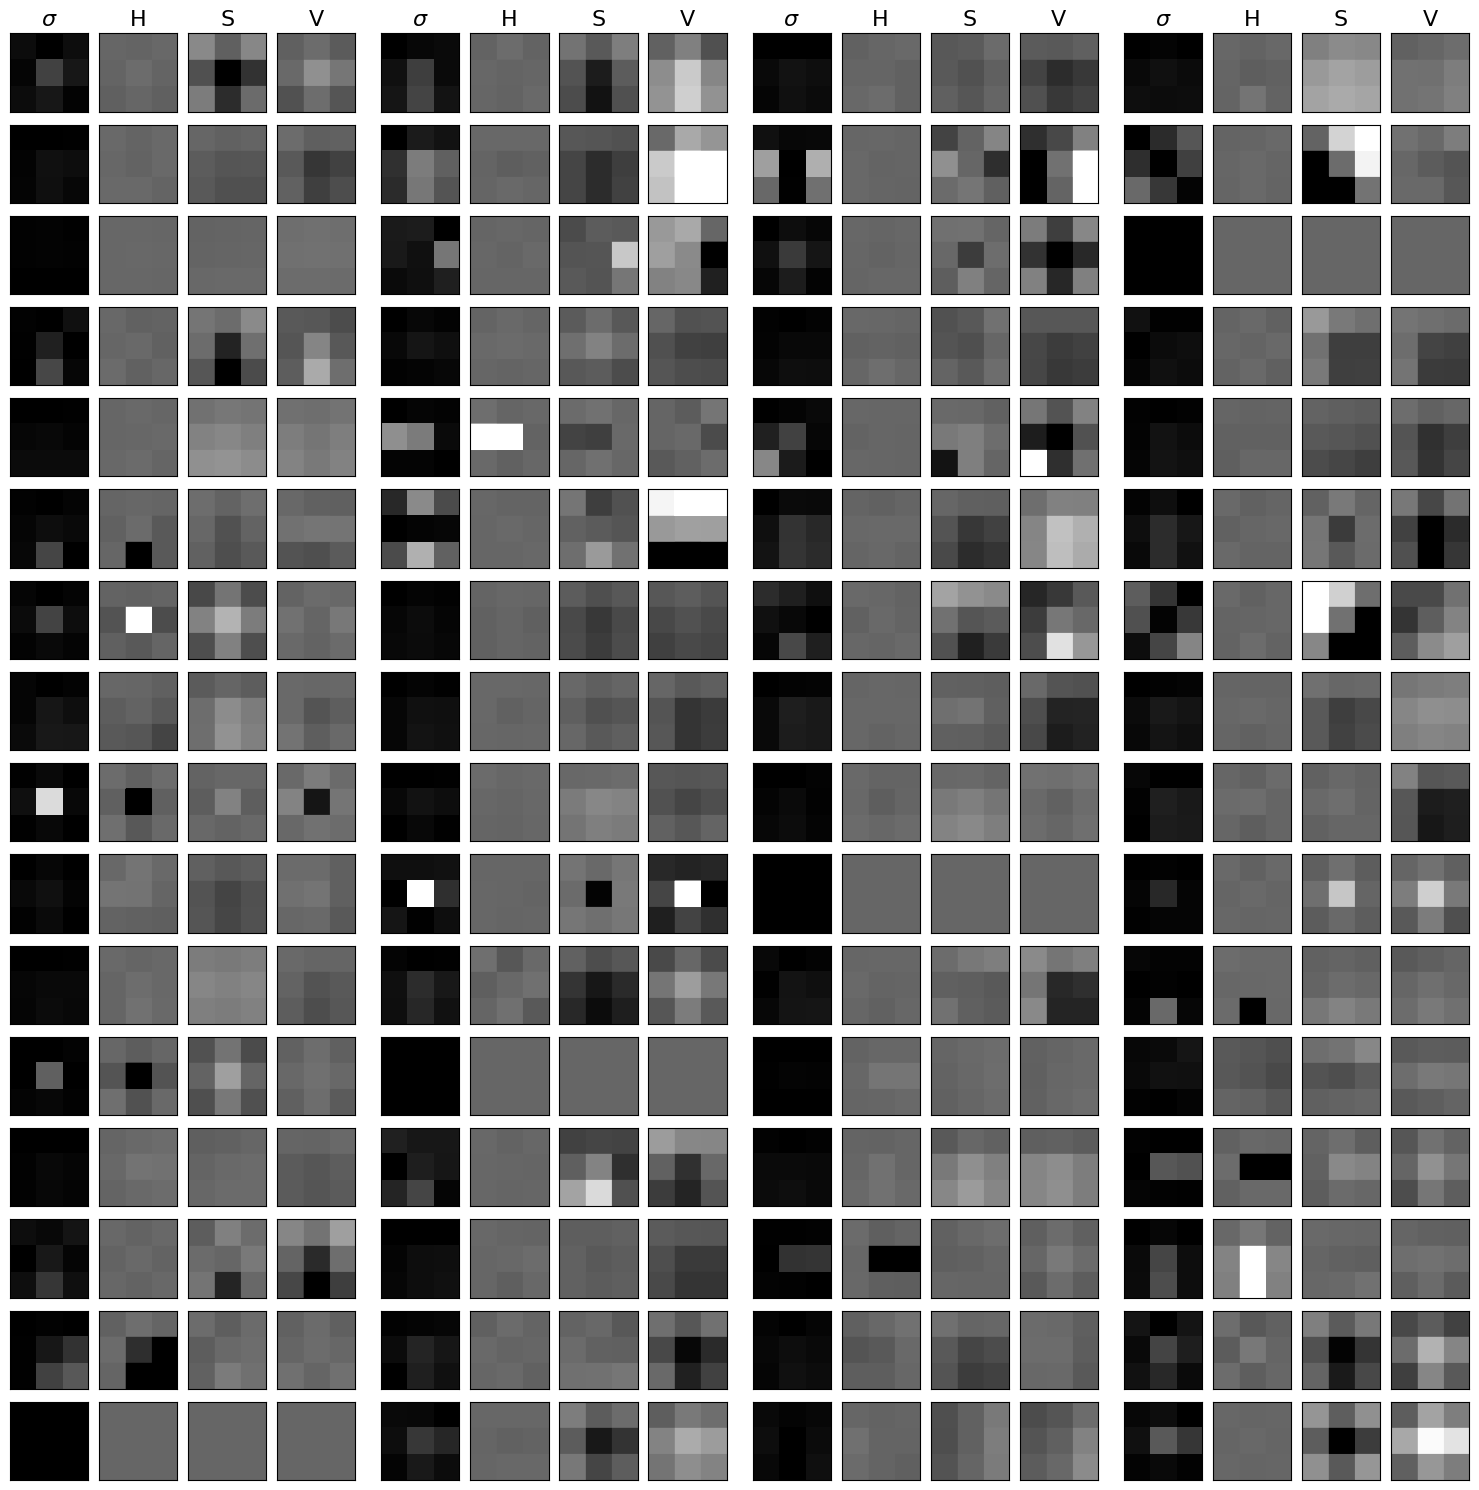}
          \caption{\scriptsize{R18 ``color-cleaned" WebFace4M (HSV)}}\label{wf4mhsv}
          \vspace{0.5em}
      \end{subfigure}
  \end{subfigure}
  \begin{subfigure}[b]{\linewidth}
      \begin{subfigure}[b]{0.325\linewidth}
        \centering
          \includegraphics[width=1\linewidth]{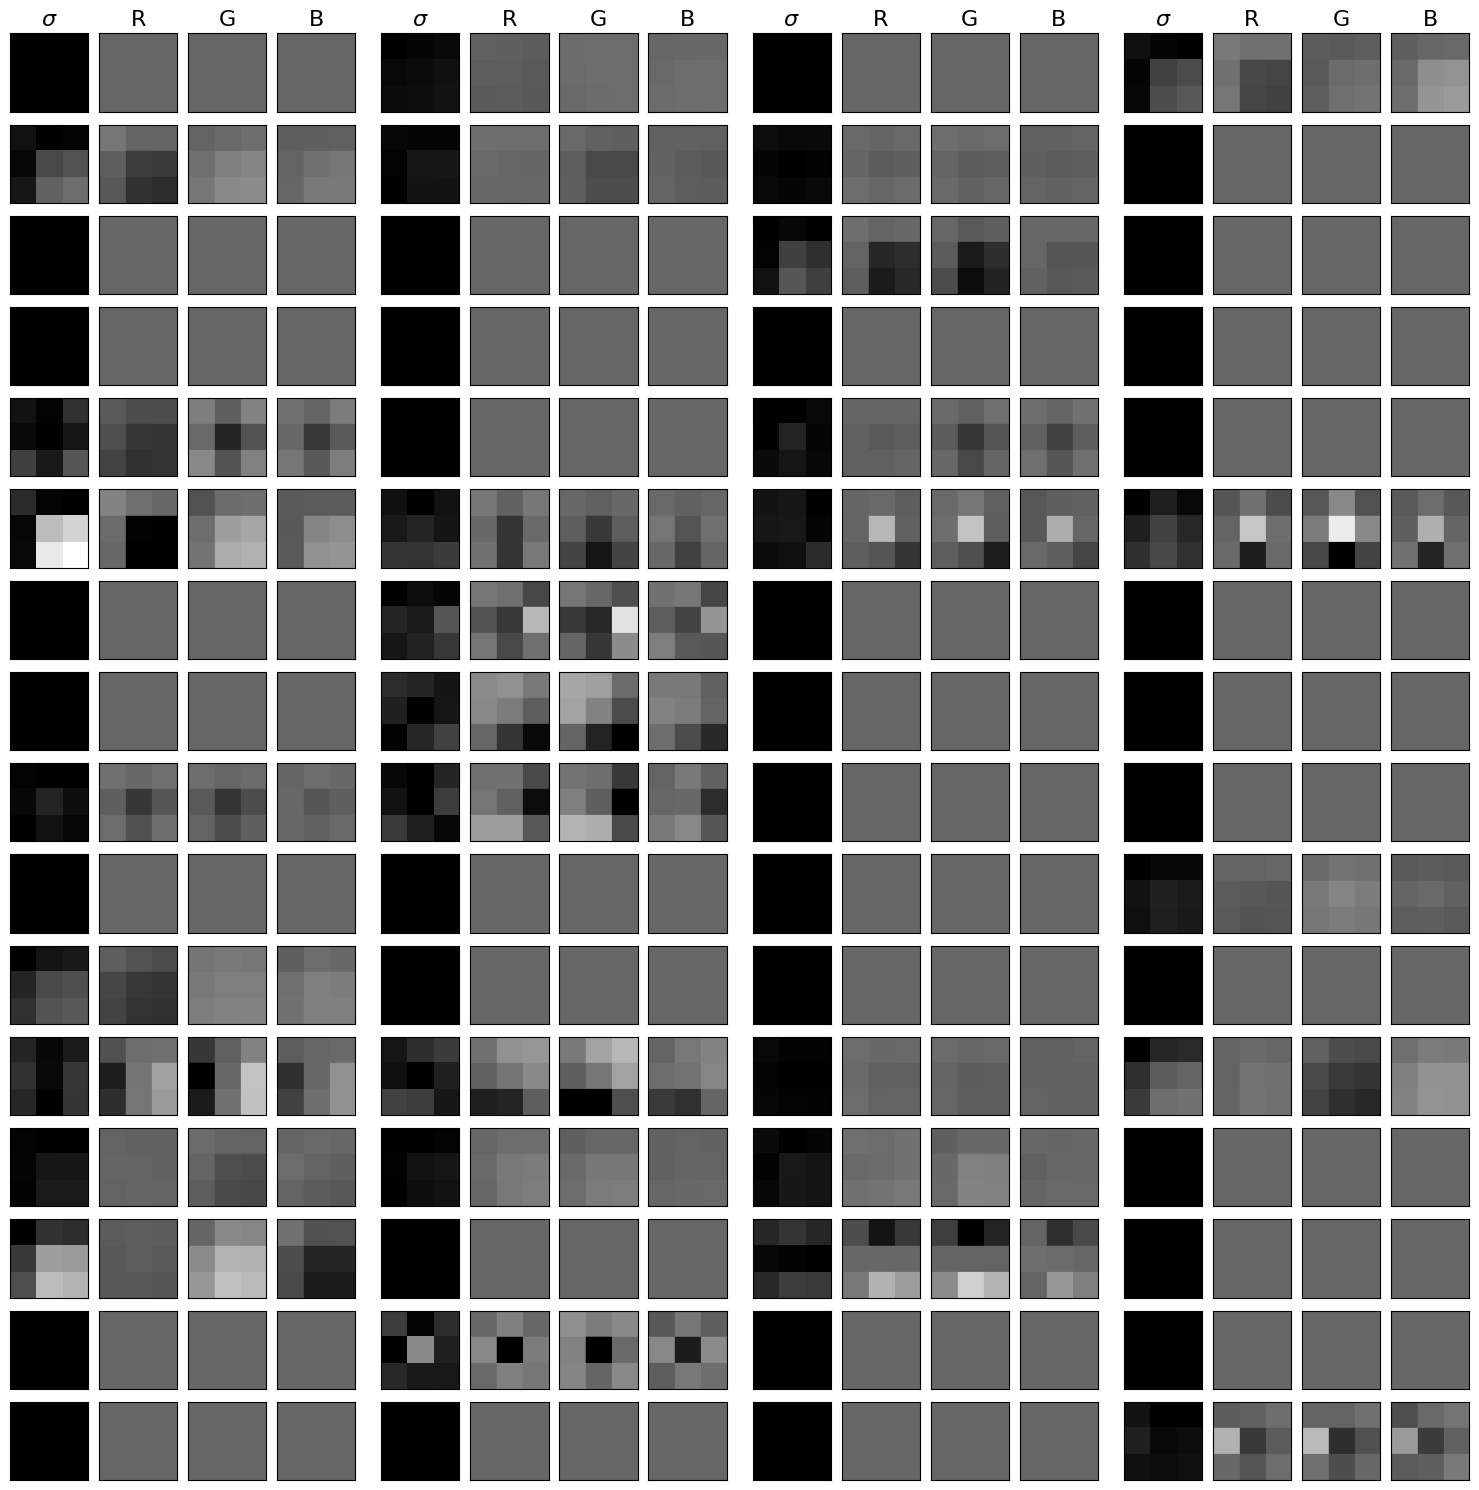}
          \caption{\scriptsize{R101 ``color-cleaned" WebFace4M (RGB)}}\label{wf4mrgb}
      \end{subfigure}
      \hfill
      \begin{subfigure}[b]{0.325\linewidth}
        \centering
          \includegraphics[width=1\linewidth]{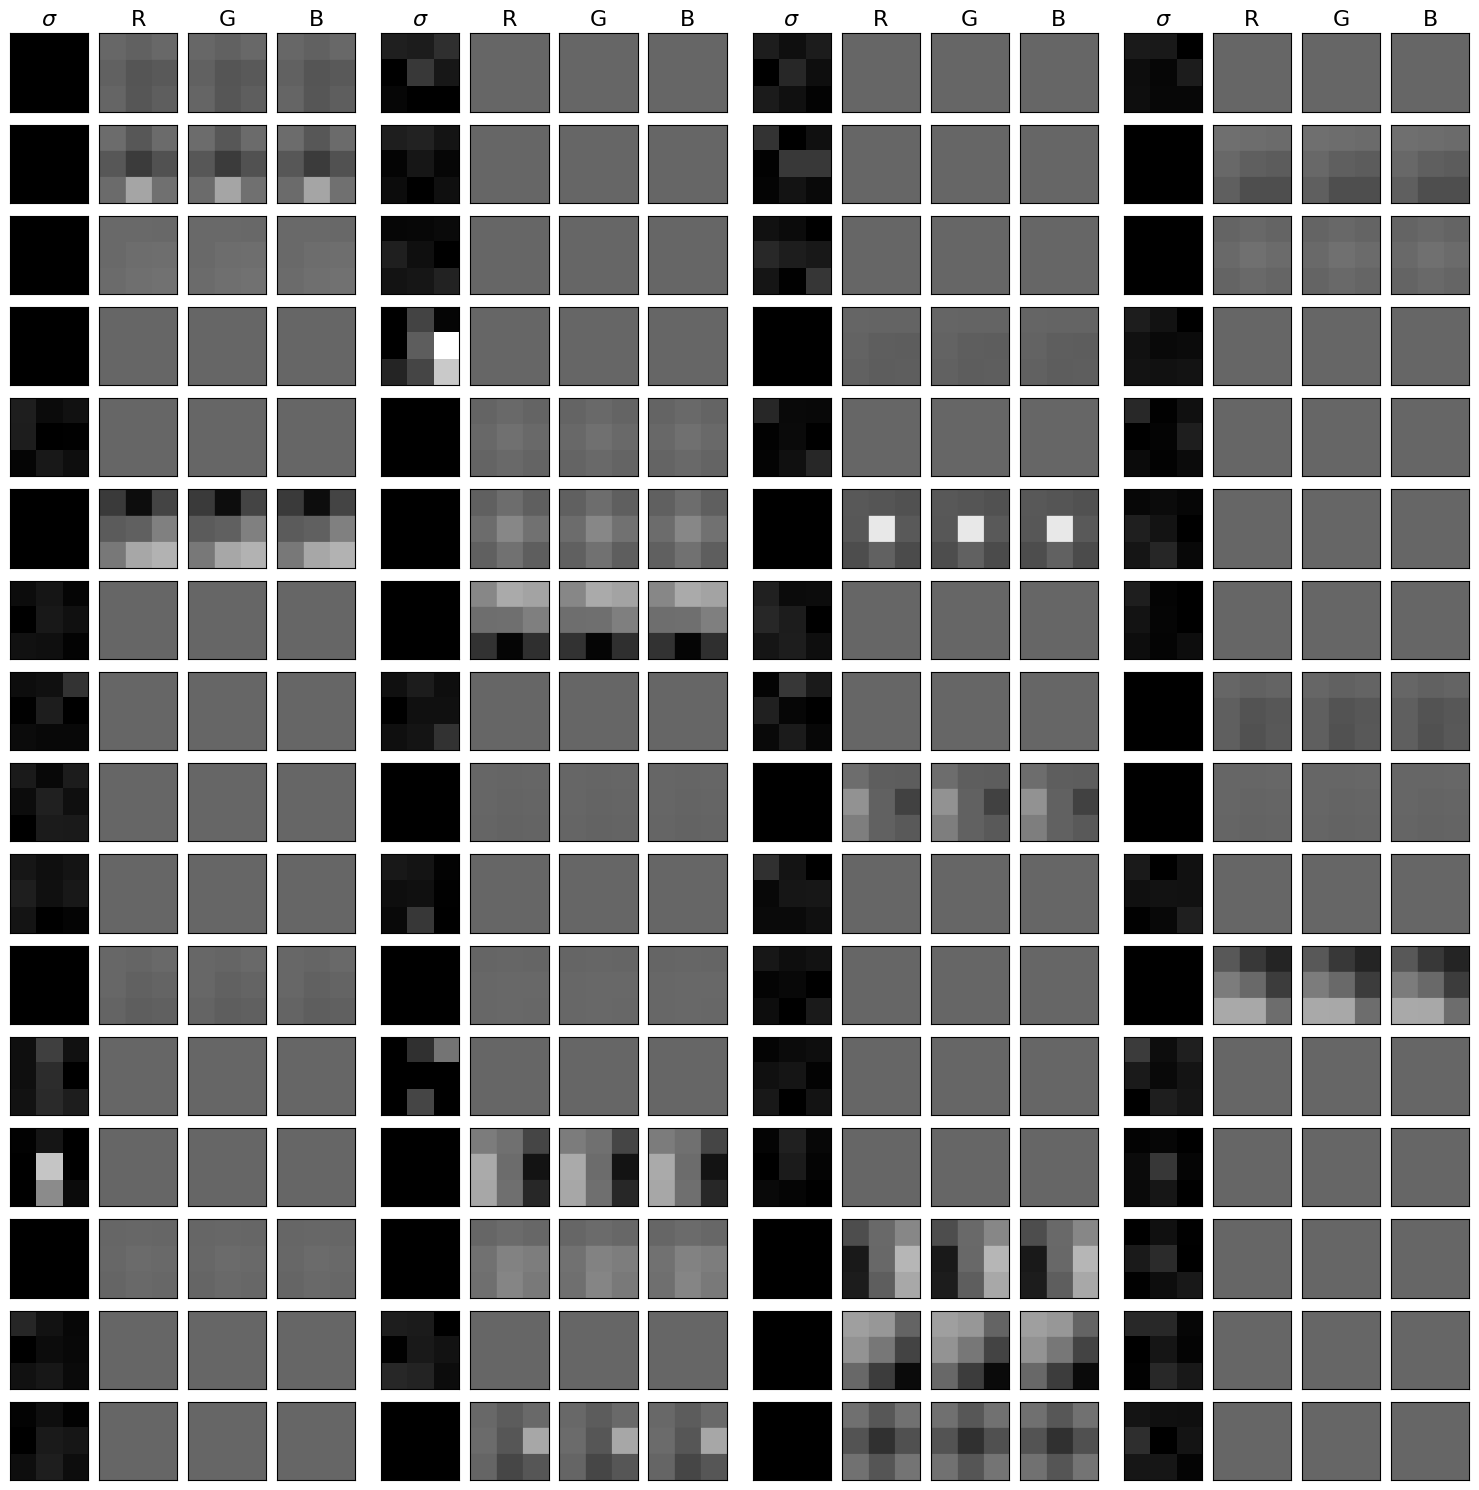}
          \caption{\scriptsize{R101 ``color-cleaned" WebFace4M (Gray 3-channel)}}\label{wf4mgray}
      \end{subfigure}
      \hfill
      \begin{subfigure}[b]{0.325\linewidth}
        \centering
          \includegraphics[width=1\linewidth]{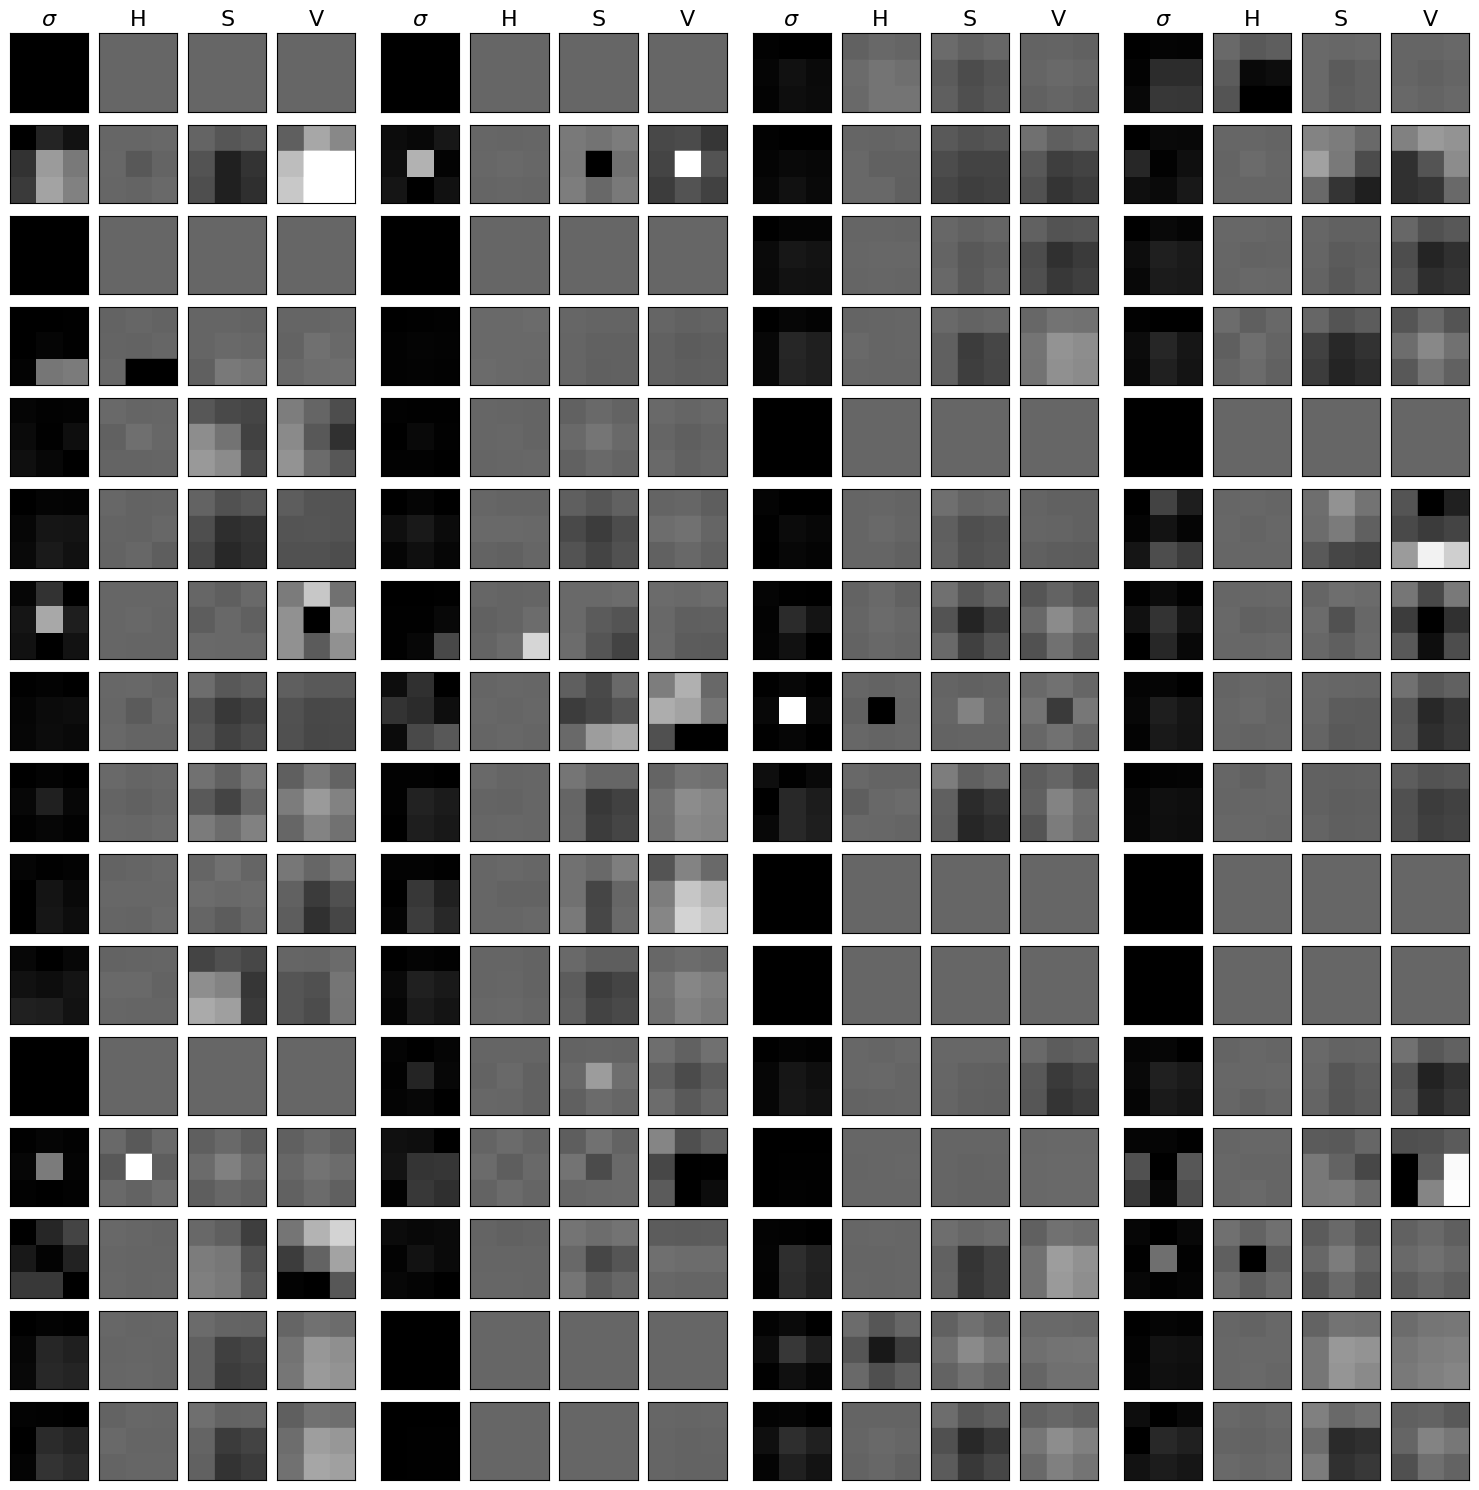}
          \caption{\scriptsize{R101 ``color-cleaned" WebFace4M (HSV)}}\label{wf4mhsv}
      \end{subfigure}
  \end{subfigure}

  \caption{\textbf{Visualization of 64 Convolution Filter Weight Values of the First Convolution Block in row-major order.} The top row shows the visualizations for trained ResNet-18 models, and the bottom row shows the visualization for trained ResNet-101 model.}
  \label{fig:weight_vis}
  \vspace{-1em}
\end{figure*}
