# Supplementary material for: What's color got to do with it? Face recognition in grayscale
Source: arXiv:2309.05180 source file (2024-07-03)
Supplement: Supplementary file 2 [file results_table_appendix.tex]

\setlength\extrarowheight{2pt}
\begin{table}[ht!]
\caption{\textbf{Training using WebFace4M vs ``color-cleaned" WebFace4M }. To obtain ``color-cleaned" WebFace4M, 300K images were dropped, but it has same performance as WebFace4M. Backbone: ResNet-50
}
\centering
\resizebox{0.98\columnwidth}{!}{
\begin{tabular}{|l|l|l|ccccc|c|}
\hline
        & \multicolumn{2}{c|}{Training Dataset} & \multicolumn{5}{c|}{Test dataset} & \\
\cline{2-9}
Model   & Type of       & Colorspace            & LFW     & CFP-FP &AGEDB-30& CALFW   & CPLFW   & Mean \\ 
Loss    & WebFace4M     & (Channels)            & [\%]    &   [\%] & [\%]   &  [\%]   &  [\%]   &  [\%] \\ 
\hline
 &       & RGB (3)               & 99.82   & 99.10  & 97.95  & 96.15   & 94.13   & 97.43\\
        & Entire              & Grayscale (3)         & 99.82   & 98.94  & 97.77  & 96.02   & 94.10   & 97.33\\
       ArcFace &               & Error$^* \rightarrow$ & \textcolor[HTML]{C41E3A}{\bf 0.00}    &  0.16  &  0.18  &  0.13   & 0.03    &  0.10\\ \cline{2-9}
        &  & RGB (3)               & 99.80   & 99.04  & 97.88  & 96.02   & 94.18   & 97.38\\
        & Color Cleaned              & Grayscale (3)         & 99.82   & 98.98  & 97.70  & 96.01   & 94.20   & 97.34\\
        &               & Error$^* \rightarrow$ & \textcolor[HTML]{C41E3A}{\bf -0.02}   & 0.06   & 0.18   & 0.01    & \textcolor[HTML]{C41E3A}{\bf -0.02}   &  0.04\\ 

\hline\hline
        &        & RGB (3)               & 99.76   & 98.94  & 97.63  & 95.95   & 94.30   & 97.32\\
        & Entire                & Grayscale (3)         & 99.76   & 98.82  & 97.51  & 95.83   & 93.78   & 97.14\\
  AdaFace      &               & Error$^* \rightarrow$ &  \textcolor[HTML]{C41E3A}{\bf 0.00}   &  0.12  &  0.12  &  0.12   &  0.52   &  0.17\\ \cline{2-9}
        &  & RGB (3)               & 99.80   & 98.81  & 97.66  & 95.96   & 94.30   & 97.31\\
        &  Color Cleaned             & Grayscale (3)         & 99.68   & 98.58  & 97.36  & 96.00   & 93.88   & 97.10\\
        &               & Error$^* \rightarrow$ &  0.12   &  0.23  & 0.30   & \textcolor[HTML]{C41E3A}{\bf -0.04}  &  0.42   & 0.20 \\ 
\hline

\end{tabular}
}

\vspace{0.1cm}

$^*$ Relative error of the accuracies computed as  (RGB - Grayscale)

\label{tab:results}
\vspace{-1em}
\end{table}
